# Supplementary material for: OmniSR: Shadow Removal under Direct and Indirect Lighting
Source: arXiv:2410.01719 source file (2025-02-10)
Supplement: Supplementary file 1 [file X_suppl.tex]

\clearpage

\setcounter{section}{0}
\setcounter{figure}{0}
\setcounter{table}{0}
\setcounter{page}{1}

\title{\vspace{-0.5em}-- Supplementary Material --\\OmniSR: Shadow Removal under Direct and Indirect Lighting}

% \maketitlesupplementary
\maketitle

\noindent{In the supplementary material we present the following:}
\begin{itemize}%[topsep=3pt]
    \item Implementation details and parameters
    \item Additional experiments and ablations
    \item Applications
\end{itemize}

\begin{algorithm*}[!t]
% \begin{multicols}{2}
\caption{Algorithm for rendering direct and indirect lighting w/ and w/o shadow.}
\label{alg:rendering}
\SetKwFunction{FDirectLighting}{DirectLighting}
\SetKwFunction{FBounceRadiance}{BounceRadiance}
\SetKwFunction{FEstimateDirectLighting}{EsteDirLight}
\SetKwFunction{FEstimateIndirectLighting}{EstIndirLight}
\SetKwFunction{FEstimateRadiance}{EstRadiance}
\SetKwProg{Fn}{Function}{:}{}

\Fn{\FEstimateDirectLighting{$p, \omega_o, with\_shadow$}}
{
    $L$ = $p$.emittedLight($\omega_o$)\;
    
    $L', \omega_i, pdf$ = lights.sampleDirection($p,\omega_o$)\;
    $is\_shadow\_ray$ = scene.isShadowIntersection($p,\omega_i$)\;
    \If {$with\_shadow = False$  or $is\_shadow\_ray = False$}
    {
        $L$+=$L'\cdot p\mathrm{.brdf}(\omega_i, \omega_o)\cdot \mathrm{cos}(\theta) / pdf$\;
    }
    return L\;
}
\Fn{\FEstimateIndirectLighting{$p, \omega_o, with\_shadow, ray\_length, bounce$}}
{
    $L$=$p$.emittedLight($\omega_o$)\;
    \If{$L$ \textgreater 0}
    {
        \tcp{ignore direct lighting from a light source}
        \lIf{bounce $\textgreater$ 1} 
        {
            return $L$ 
        }
        \lElse
        {
            return 0
        }
    }
    $\omega_i, pdf, brdf$ = $p$.brdf.sampleDirection($\omega_o$)\;
    \If{$with\_shadow$ = False and $bounce=1$}
    {
         \If{$ray\_length \leq r$ or $\mathrm{mod}(trans\_depth, 2) = 1$}
         {
         	$\omega_i = -\omega_o, brdf = 1$\;
         	$trans\_depth$+=1; \tcp{\# of transparent intersections}
         }
     }

    $p'$=IntersectScene($p, \omega_i$)\;
    $cpdf$ = continuationProbability($p.brdf, \omega_i, \omega_o$)\;

    \If{$\mathrm{random01}()$ $\leq$ cpdf}
    {
        $L$+=\FEstimateIndirectLighting($p', -\omega_i, with\_shadow, \mathrm{length}(p, p'), bounce+1$)$\cdot \frac{brdf \cdot\mathrm{cos}(\theta)}{pdf\cdot cpdf}$\;
    }
    
    return L
}

\Fn{\FEstimateRadiance{$x,\omega,with\_shadow,bounce=0$}}
{
    $p$=IntersectScene($x, \omega$);\tcp{a ray traced from the camera position $x$ along direction $\omega$, intersecting the scene at point $p$}
 
    return \FEstimateDirectLighting($p, -\omega, with\_shadow$)+
    
        $\qquad$ max(\FEstimateIndirectLighting($p, -\omega, with\_shadow, \mathrm{length}(x, p), bounce$),
        
        $\qquad$ \FEstimateIndirectLighting($p, -\omega, True, \mathrm{length}(x, p), bounce$))\;
}
% \end{multicols}
\end{algorithm*}

\begin{algorithm*}[!t]
\caption{Algorithm for camera selection.}
\label{alg:view_selection}
\LinesNotNumbered
  \SetKwInOut{Input}{input}\SetKwInOut{Output}{output}

  \Input{The scene set $\mathcal{S}=\{S_i\}$,
    each $S_i$ contains a set of rooms $\mathcal{R}_i=\{R_j\}$, and each $R_j$ contains a set of furniture $\mathcal{F}_j=\{F_k\}$
  }
  \Output{The camera pose set $\mathcal{P}$}
  \BlankLine
  
\ForEach{$S_i$ in $\mathcal{S}$}
{  
    remove $R_j$ whose $\left|\mathcal{F}_j\right| < 5$ from $\mathcal{R}_i$ \;
    \ForEach{$R_j$ in $\mathcal{R}_i$}
    {
        \For{$n\leftarrow 1$ \KwTo $N$}
        {
            \For{$m\leftarrow 1$ \KwTo $2000$}
            {
                sample $t_n(x,y,z)$ s.t. $t_n$ \emph{in} $R_j$ \emph{and} $z \in [1.2,1.8]$\;
                sample $r_n(pitch,yaw,roll)$ s.t. $roll=0^ {\circ},pitch\in[60^ {\circ},120^ {\circ}],yaw\in[0^ {\circ},180^ {\circ}]$\;
                $P_n \leftarrow \{r_n, t_n\}$\;
                $p, d=\mathrm{hit}_{surf}(L_n, R_j)$; \tcp{$p$ is the intersection of the camera's optical axis $L_n$ and the room, $d$ is the distance}
                
                \If{$p$ in $R_j$ and $d\in[1.0, 5.0]$}
                {
                    $\mathcal{L} \leftarrow$ uniformly sample $M$ ray in the viewport\;
        
                    $\{M_{F_k}\}=\mathrm{hit}_{obj}(\mathcal{L}, \mathcal{F}_j)$;\tcp{$M_{F_k}$ is the number of intersections with furniture ${F_k}$}
    
                    \If{$\max(\{M_{F_k}\})/M \leq 0.3$ and $\sum\limits_k{M_{F_k}}/M$ in $[0.35,0.8]$}
                    {
                        add $\left<R_j,P_n\right>$ to $\mathcal{P}$\;
                        break\;
                    }
                }   
            }
        }
    } 
}
\end{algorithm*}

\section{Implementation Details}  
\label{sec:imp}

\subsection{Shadow and shadow-free image rendering.}

We render shadow and shadow-free images via path tracing, as outlined in Algorithm \ref{alg:rendering}. In this process, the final radiance comprises both direct lighting and indirect lighting. The shadow-free radiance is obtained by rendering with the setting $with\_shadow=False$.

Specifically, the radiance of direct lighting is computed using the function \CommentSty{EsteDirLight}$(\cdot)$. In the case of $with\_shadow = True$, if the direct lighting $L'$ originating from a light source and reaching the first intersection point $p$ is obstructed, we disregard the radiance from that light source. Conversely, when $with\_shadow = False$, the obstructed radiance $L'$ is included, resulting in a shadow-free radiance.

On the other hand, the indirect lighting's radiance is calculated through the \CommentSty{EstIndirLight}$(\cdot)$ function in Algorithm \ref{alg:rendering}. This process involves recursively tracing the light path
until it reaches a light source or randomly terminates using the Russian Roulette method. The variable $bounce$ will be increased after each ray-surface intersection. When rendering the radiance due to indirect lighting, if a light path reaches a light source and the $bounce \leq 1$, the radiance from that light source is set to zero. If $with\_shadow = False$, when dealing with a ray at $bounce = 1$ along the light path, we will consider the intersection $p$ as ``transparent'' if it falls within a threshold $r$. In this context, ``transparent'' signifies that the ray will pass through $p$ in the same direction, with a BRDF of 1. To prevent the ray from intersecting inner surfaces, we will designate the next intersection as ``transparent'' if $trans\_depth$ is an odd number. Here, $trans\_depth$ represents the count of previous transparent intersections, assuming all furniture is watertight. Notably, the first intersection at the first bounce from a point will be preserved if it is the last intersected object, even when its distance is within 1 meter, such as walls or ceilings. Finally, the ultimate shadow-free image is calculated by taking the per-pixel maximum value between an indirect-lighting image without shadows and indirect-lighting image with a shadow.

The rendering process described above was implemented using the Blender Cycles engine \cite{blender} and Open Shading Language (OSL). The samples of our rendering results, including the shadow image, shadow-free image, and shadow probability map, are illustrated in Fig.~\ref{fig:supp_dataset}.

\subsection{Camera and light selection.}

\begin{figure}[t]
\centering
\includegraphics[width=\linewidth]{./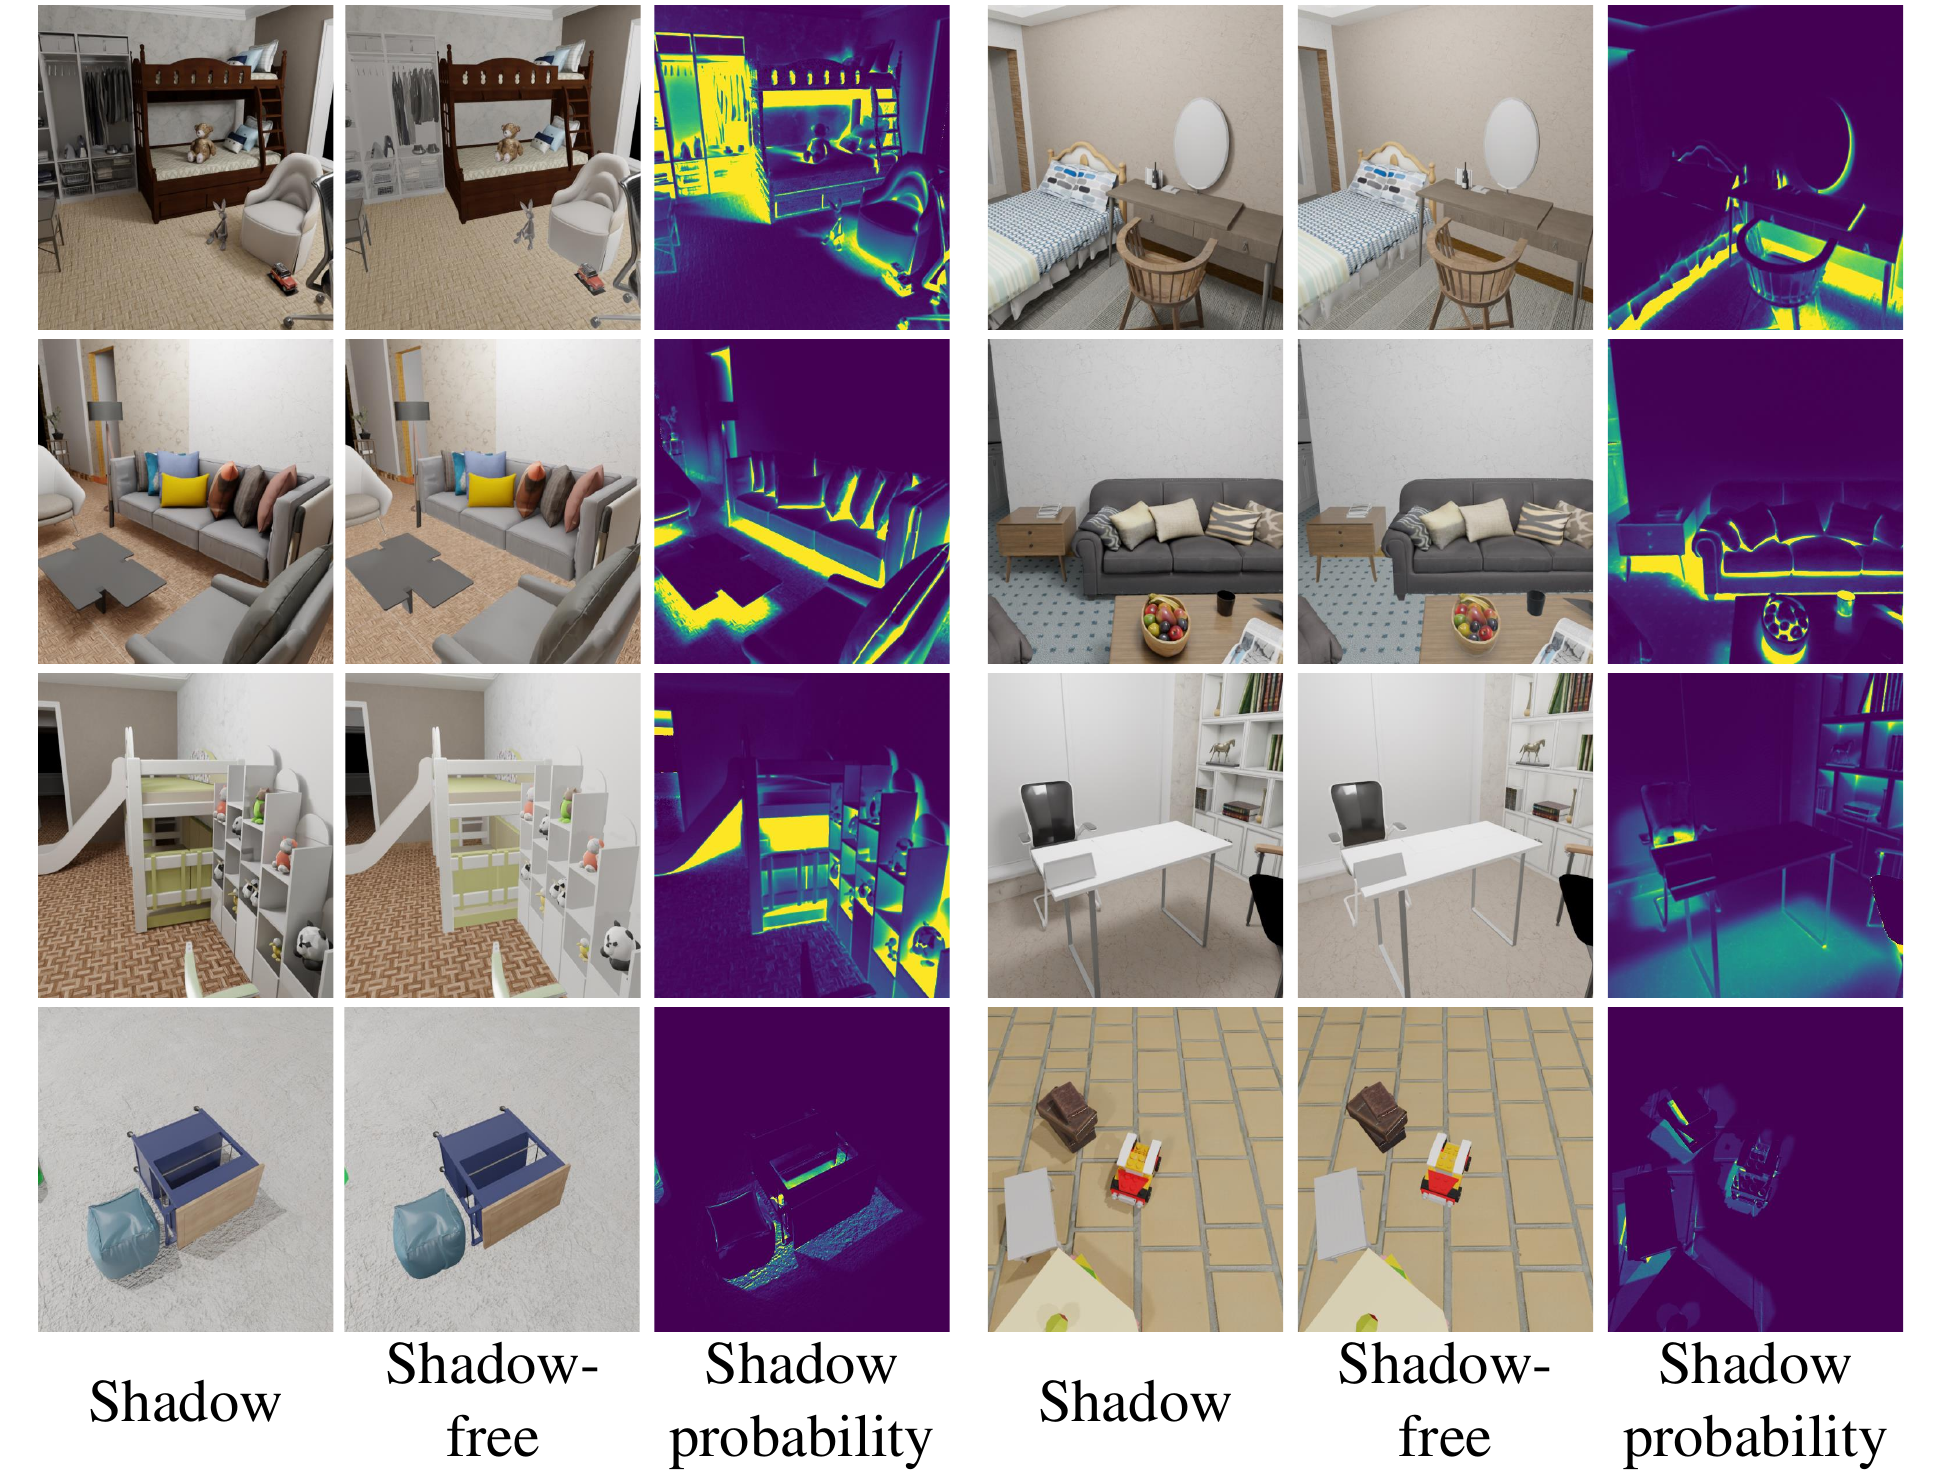}
\caption{\textbf{Samples of our rendering results} including the shadow image, shadow-free image, and shadow probability map.
}
\label{fig:supp_dataset} 
\end{figure}
\begin{figure}[t]
\centering
\includegraphics[width=\linewidth]{./fig/light_sources.png}
\caption{\textbf{Illustration of light sources and scenes in the 3DFront~\cite{fu20213dfront} dataset}.} 
\label{fig:light_sources}
\end{figure}

\paragraph{Camera selection.} As a pre-processing step in rendering our dataset, the algorithm for camera (view) selection is outlined in Algorithm~\ref{alg:view_selection}. For a given scene $S_i\in\mathcal{S}$, we iterate through all the rooms within $S_i$ that contain five or more pieces of furniture. Within each room meeting this criterion, we aim to select $N$ valid cameras, if possible. In our experiments, we set $N$ as 2.

Specifically, we randomly select a camera location $t_n(x, y, z)$ within the room's bounding box, where the height $z$ ranges between 1.2 and 1.8 meters. Subsequently, we sample a camera rotation $r_n$ with a zero roll and a pitch between 60 and 120 degrees. The central intersection point denoted as $p$ represents the point where the camera's optical axis intersects the scene. 

The validity of the sampled camera is contingent upon the following criteria: 1. The central intersection of the viewport ($p$) must remain within the room and maintain a suitable distance from the camera (between 1 and 5 meters). 2. The furniture occupancy within the viewport should avoid extreme sparsity or overcrowding, aiming for an occupancy rate between 35\% and 80\%. Notably, ``furniture'' excludes elements such as the cell, wall, and floor. 3. No single piece of furniture dominates the entire viewport, exceeding 30\% of the viewport.

\paragraph{Light selection.} For each room $R_j$ and selected camera $P_n$, our algorithm next determines whether to activate existing light sources or insert new ones. Initially, we retrieve all light sources according to the class labels and deactivate them. Subsequently, we activate those light sources positioned within the room and near the central intersection of the viewport ($p$), specifically those whose centroids are within a 2.5-meter distance. Here, distance is defined as the 2D distance measured along the $xy$ plane. Note that the light sources in 3DFront dataset~\cite{fu20213dfront} are not point light source or area light source, but lamp with complex geometries, as depicted in Fig.~\ref{fig:light_sources}. 

In cases no light sources are found near the intersection point $p$, we implement a solution by randomly inserting a ceiling lamp in the area. We achieve this by randomly selecting a lamp from the 3DFront dataset's asset collection and positioning it at a random $xy$ coordinate within a 2.5-meter distance from the intersection point $p$ and within the room. We then adjust the lamp's $z$ coordinate to align it flush with the ceiling. Additionally, we add a random point light located between 1 and 4 meters from $p$, near the ceiling and outside the viewport. This addition enriches the variety of shadow within the space.

\paragraph{Object composition scenes.} 

For the object composition scenes, we create a cube-shaped room with each surface measuring $10 \times 10$ meters. We then randomly sample objects from the ABO~\cite{collins2022abo} and Objaverse~\cite{deitke2023objaverse} datasets, with each object rescaled to a size between 0.5 and 1.0 meters. These objects are positioned either directly on the floor or slightly above it. For the lighting, we randomly select 1 to 2 area lights and 1 to 2 spotlights, ensuring all light sources remain invisible.

\paragraph{Shadow mask.} 

After obtaining shadow image $\mathbf{I}_s=\mathbf{I}^{dr}_s+\mathbf{I}^{idr}_s$ and shadow-free image $\mathbf{I}_f=\mathbf{I}^{dr}_f+\mathbf{I}^{idr}_f$, the probabilistic shadow mask $\mathbf{S}$ is defined as:
\begin{align}
\label{equ:shadow_prob}
\mathbf{S}=\mathrm{clip}(\left( \mathbf{I}_f-\mathbf{I}_s \right) /\mathrm{max}(\mathbf{I}_f,0.1)).
\end{align}
Here, $\mathrm{clip}(\cdot)$ clips the results within the range of $[0, 1]$. For real images with noise, a clipping threshold of 0.1 is applied to $\mathbf{I}_f$ to prevent the near-black areas from being easily misclassified as shadows.

\subsection{Scene rearrangement.}

As shown in Fig. \ref{fig:scene_rearrangement}, the 3DFront~\cite{fu20213dfront} scenes exhibit unwanted penetrations and collisions, which can adversely affect the realism of the dataset. To mitigate this, we introduce a local object rearrangement method to address this issue.

\begin{figure}[t]
\centering
\includegraphics[width=\linewidth]{./fig/scene_rearrangement.png}
% \vspace{-0.5cm}
\caption{\textbf{Examples of before/after rearrangement}. Our rearrangement procedure resolves unwanted collisions, as indicated by the red arrow.}
\label{fig:scene_rearrangement} 
% \vspace{-0.2cm}
\end{figure}

\begin{figure}[t]
\centering
\includegraphics[width=0.8\linewidth]{./fig/supp_rearrangement.png}
\caption{\textbf{Procedure for scene rearrangement}. 
To address collisions between the furniture (indicated by the red box) and the wall (indicated by the black box), we utilize a spiraling outward movement. The first non-colliding position is highlighted within the dashed red box.}
\label{fig:supp_rearrangement} 
\end{figure}

The aim of scene rearrangement is to resolve furniture collisions within the original 3DFront dataset~\cite{fu20213dfront}. These collisions are identified using 3D intersection queries between furniture and walls, leveraging the CGAL library \cite{cgal}. To expedite the search process, we confine furniture movement to the 2D $xy$ space. During the scene rearrangement phase, our approach selectively relocates or removes furniture, while maintaining the fixed positions of the walls.

We first sort all furniture in ascending order by the area of their 2D bounding boxes. This ensures that smaller furniture is prioritized for relocation or removal. During rearrangement, if a piece of furniture $F_i$ intersects with other furniture or walls, we employ a spiraling outward movement for $F_i$ in concentric loops (Fig.~\ref{fig:supp_rearrangement}). This movement is limited to a maximum radius of 0.5 meters.

At each position along this outward spiral, we check for collisions between $F_i$ and other furniture or walls. If a safe position is found, we move $F_i$ there and proceed to the next furniture encountering collisions. Otherwise, if no safe position is available, we place $F_i$ at the last location and identify the smallest furniture that causes a collision with $F_i$, denoted as $F_j$. This furniture is then marked as the next item requiring adjustment. In the next iteration, similar to the process for $F_i$, we navigate $F_j$ through the same steps, attempting to find a non-colliding position. In case $F_j$ still cannot secure a collision-free position, we removing the previous furniture $F_i$, and backtrack $F_j$ to its initial placement. We iterate through this algorithm until all collisions have been resolved. 

Note that our scene rearrangement algorithm is designed specifically to address collisions rather than generate scenes. Our approach may not guarantee that all furniture adheres to a well organized layout. However, for tasks like shadow removal, some instances of non-standard layouts are acceptable.

\subsection{Network and Training details.}

Throughout the training, we maintain a batch size of 8 and terminate the process after 40 epochs for the proposed INS dataset and 500 epochs for other datasets. For the INS dataset, each batch comprised $512\times512$ patches, utilizing a Swin attention window size of 16. For other datasets, batches consisted of randomly cropped patches sized at $480\times480$, with the window size set to 15. All random seeds in our experiments are fixed at 1234.

For an image with dimensions $W\times H$, the DINO features are obtained at a resolution of $W/14 \times H/14$~\cite{oquab2023dinov2}. To generate a feature map that can concatenate with the bottleneck layer, which operates at a resolution of $W/8 \times H/8$, we initially resize the image to $W\cdot 14/8 \times H\cdot 14/8$ using bilinear interpolation, extract its DINO features, and apply a $1 \times 1$ convolution layer to obtain a feature map of size $256 \times W/8 \times H/8$.

In our experiments, we utilize distributed data parallelism (DDP) and automatic mixed precision to expedite training. Additionally, our training pipeline incorporates simple data augmentation techniques, including random rotations within a range of $-20$ to $+20$ degrees and horizontal flipping. We recognize the potential for further enhancement by exploring and integrating more sophisticated data augmentation methods.

% Please refer to the supplementary material for more details.

% We employ the distributed data parallel (DDP) to accelarate the training process. For optimization, we utilize the Adam optimizer~\cite{Kingma2015AdamAM}. The learning rate is initially set to $1\times10^{-3}$ and is adjusted using a cosine annealing~\cite{loshchilov2016sgdr} scheduler. Additionally, during training, we incorporated simple data augmentation methods, including random rotation (ranging from $-20$ to $+20$ degrees) and horizontal flipping. We believe that more sophisticated data augmentation methods can also be explored and integrated for further improvement.

\begin{figure}[!t]
\centering
\includegraphics[width=\linewidth]{./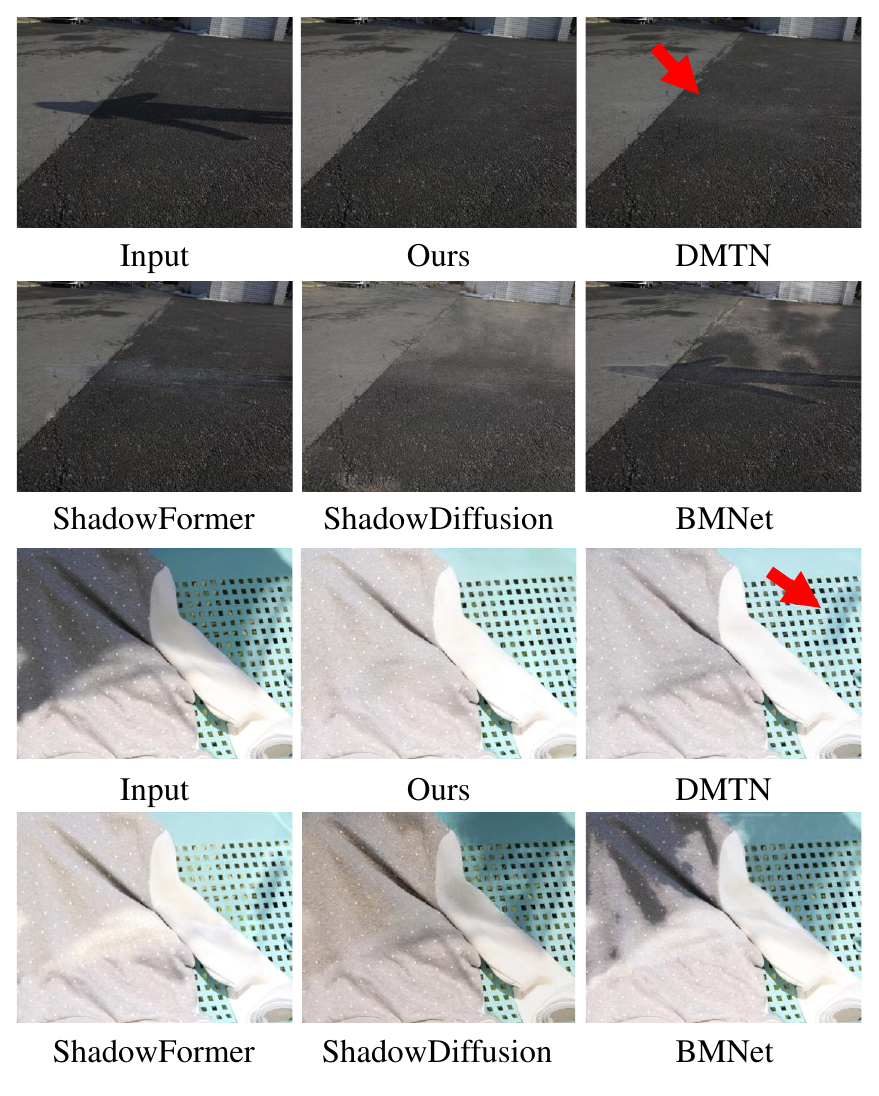}
\caption{\textbf{Comparisons with DMTN \cite{liu2023decoupled}, ShadowFormer \cite{guo2023shadowformer},  ShadowDiffusion \cite{guo2023shadowdiffusion}, and BMNet \cite{zhu2022bijective} on SRD~\cite{qu2017deshadownet} dataset.}}
\label{fig:supp_srd_comparison} 
\end{figure}
\begin{figure*}[!t]
\centering
\includegraphics[width=0.95\linewidth]{./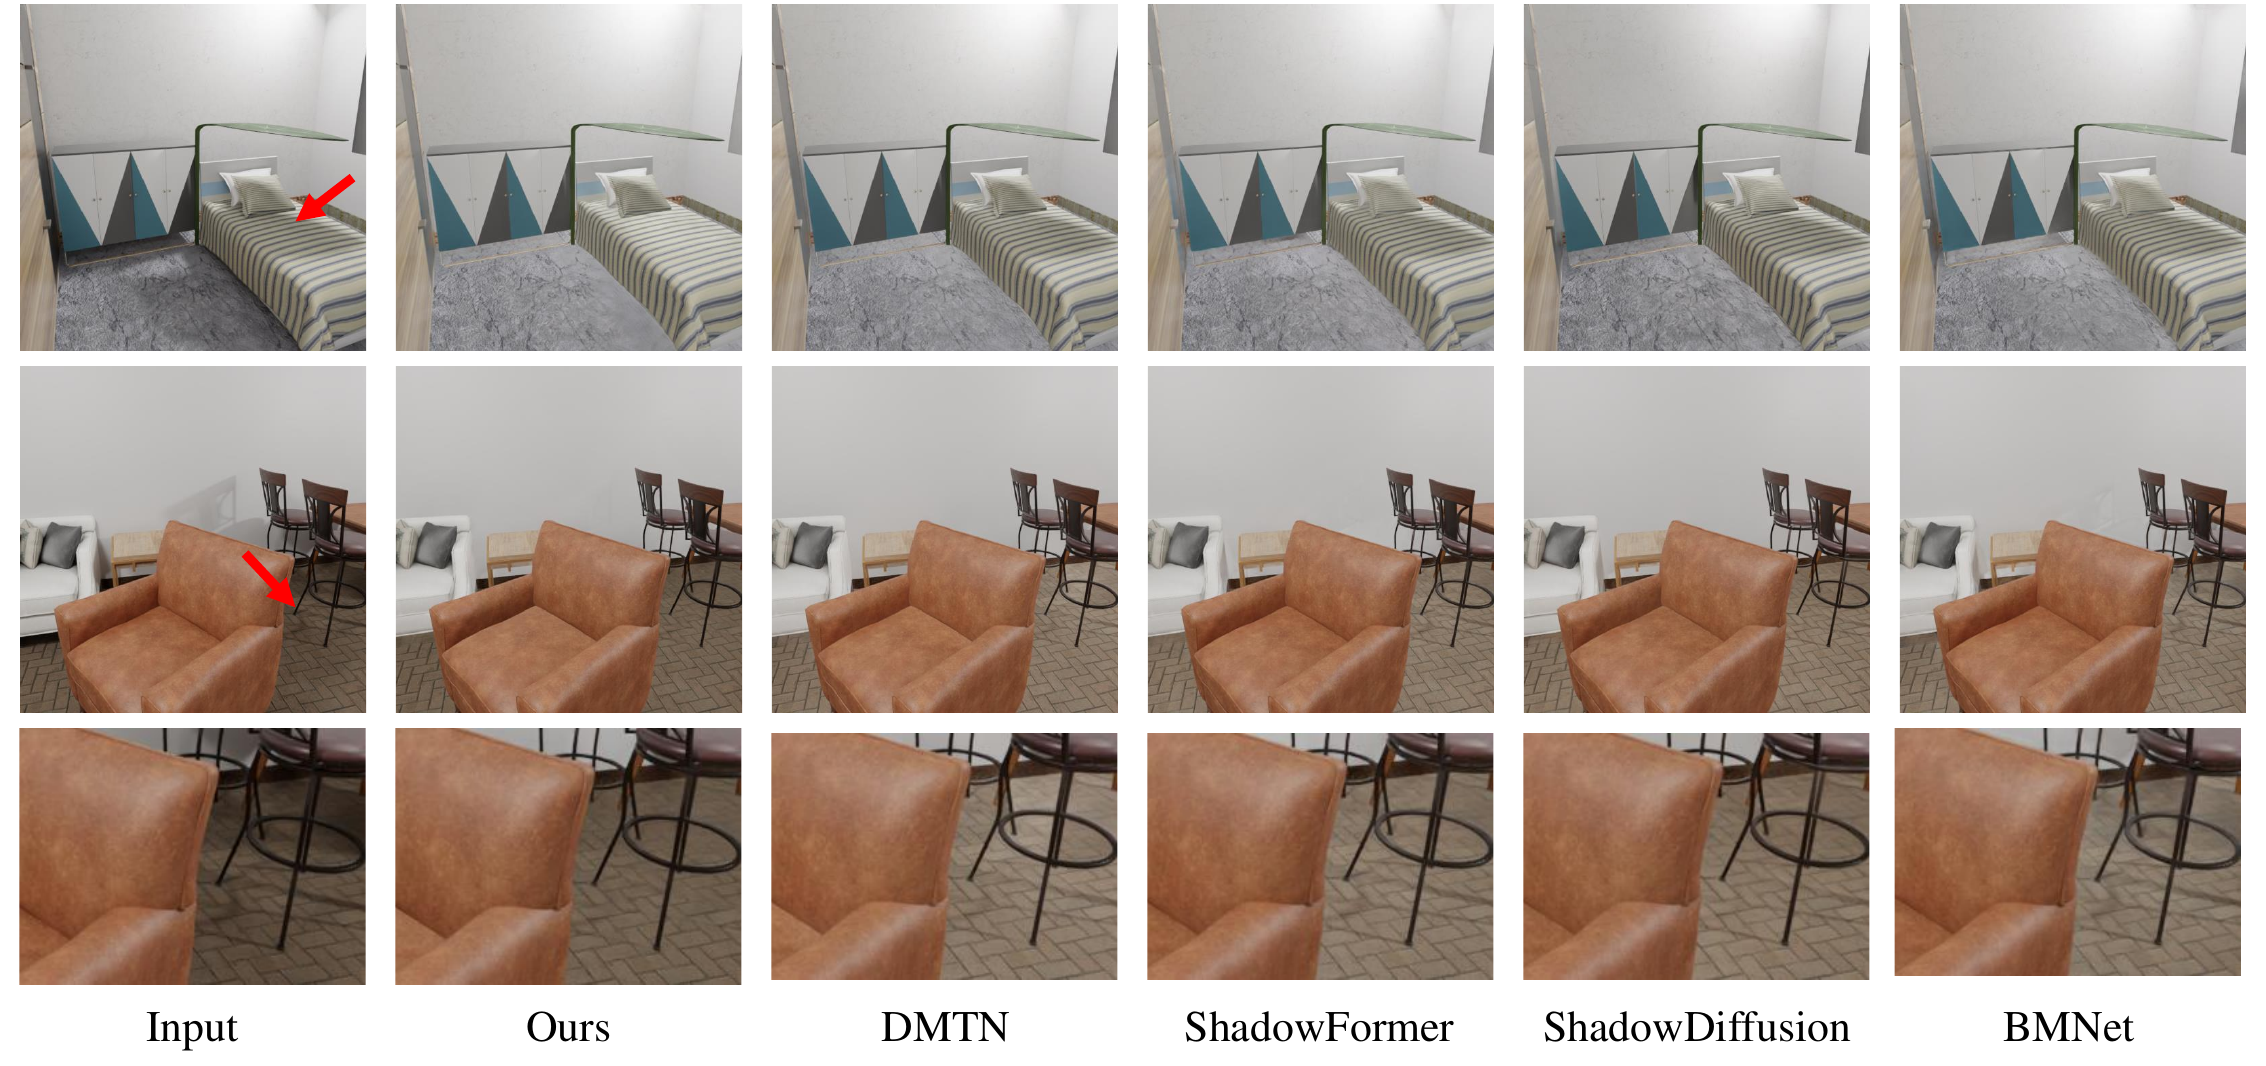}
\caption{\textbf{Comparisons on the testing data within the proposed INS dataset.}}
\label{fig:supp_ins_testing_comparison} 
\end{figure*}

\begin{figure*}[!t]
\centering
\includegraphics[width=0.95\linewidth]{./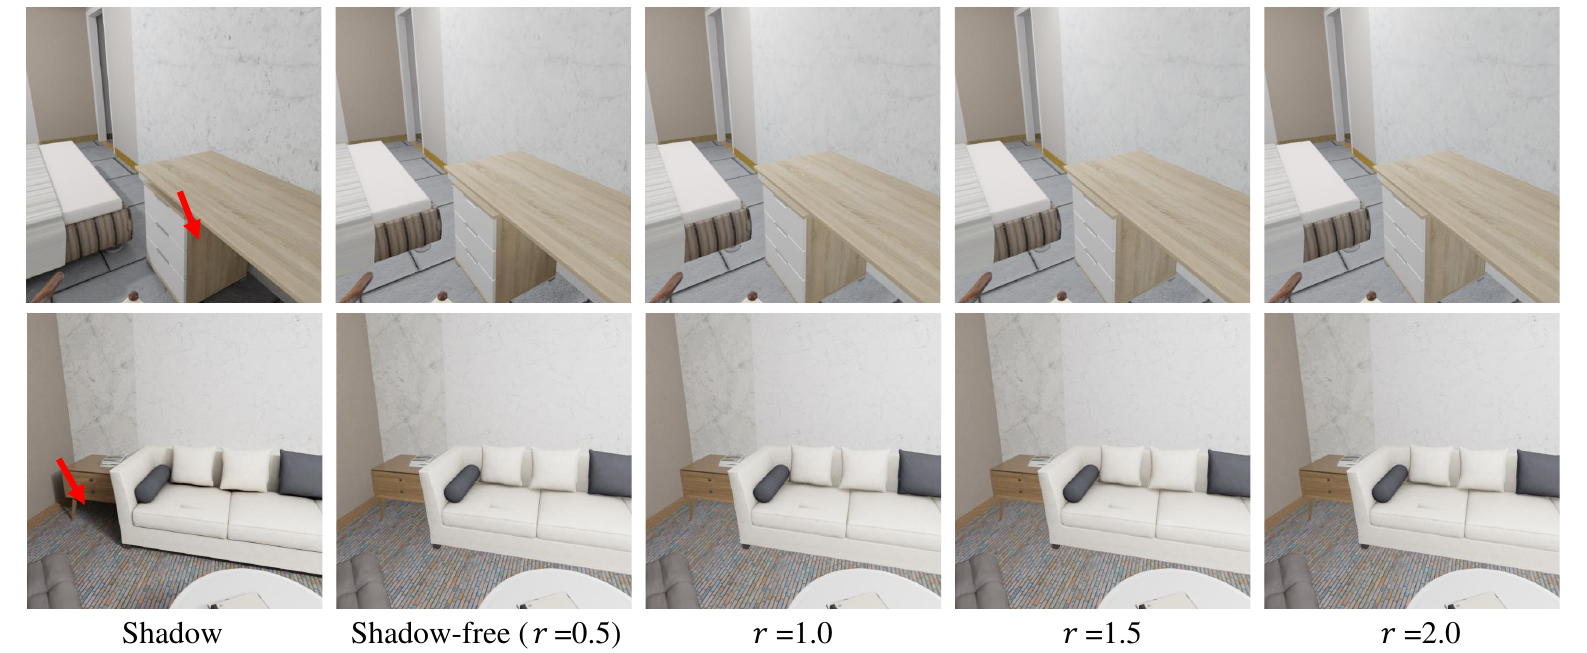}
\caption{\textbf{Rendering results on different occlusion radius $r$}.}
\label{fig:supp_different_r} 
\end{figure*}

\begin{figure*}[!t]
\centering
\includegraphics[width=0.8\linewidth]{./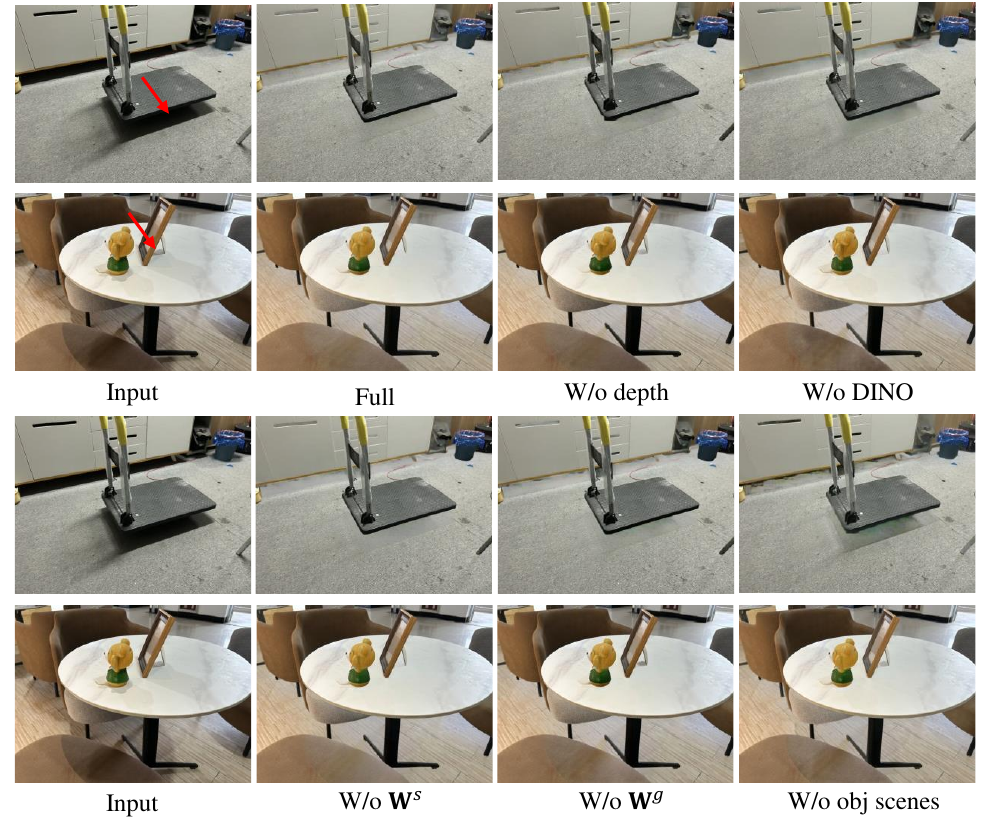}
\caption{\textbf{Results of ablation studies.}}
\label{fig:supp_ablation_comparison} 
\end{figure*}

\begin{figure*}[!t]
\centering
\includegraphics[width=1.0\linewidth]{./fig/supp_comparison.jpg}
\caption{\textbf{Additional comparisons with SOTA shadow removal methods, using real captured images.}}
\label{fig:supp_comparison_1} 
\end{figure*}

\section{Additional Experiments} 
\label{sec:exp}

\subsection{More results on the SRD dataset~\cite{qu2017deshadownet}, INS dataset, and real captured images.}

In this section, we present the comparison results on the SRD dataset~\cite{qu2017deshadownet} in Fig.~\ref{fig:supp_srd_comparison}. Our shadow removal method demonstrates the best performance compared to other methods that either utilize detected shadow masks~\cite{zhu2021mitigating} or do not require shadow masks.

We also present additional comparison results on the proposed INS dataset (Fig.~\ref{fig:supp_ins_testing_comparison}) and real captured indoor scene images (Fig.~\ref{fig:supp_comparison_1}). In contrast to DMTN \cite{liu2023decoupled}, ShadowFormer \cite{guo2023shadowformer}, ShadowDiffusion \cite{guo2023shadowdiffusion}, and BMNet \cite{zhu2022bijective}, our method excels in removing direct and indirect shadows within intricate indoor scenes. Notably, despite being trained on our synthetic dataset, our method demonstrates remarkable performance when applied to real indoor scenes, which is a crucial aspect for practical real-world applications.

\subsection{Comparisons on Different occlusion radius $r$.}

We present the comparison results for different occlusion radius $r$ in Fig.~\ref{fig:supp_different_r}. Our goal is to use a relatively small occlusion radius that can eliminate almost all indirect shadows, as a larger radius may excessively alter the indirect illumination, leading to unintended color changes in areas without occlusion. As shown in Fig.\ref{fig:supp_different_r}, $r=1$ generally outperforms $r=0.5$ in shadow regions while offering similar performance to $r=1.5$ and $r=2.0$. Consequently, we eliminate occlusions within a radius of $r=1$ along the first bounce's ray, which is sufficient to remove almost all indirect shadows in our dataset.

\subsection{Qualitative results of ablation studies.}

We present the comparison results of the ablation studies. As shown in Fig.~\ref{fig:supp_ablation_comparison}, our full model delivers the best shadow removal performance compared to the other ablation configurations. For instance, it effectively removes the shadow behind the photo frame on the white desk.

\section{Details for Applications}  
\label{sec:app}

As depicted in Fig. \ref{fig:application}, we developed two applications focused on indoor scene editing to verify the significance of our indirect shadow removal method. The first application involves shadow-preserving ControlNet-based editing \cite{zhang2023adding}. In this scenario, we eliminate shadows from the generated image and reintegrate the shadows detected from the original image. The second application, based on intrinsic decomposition \cite{li2022physically}, highlights that without shadow removal, some shadow components are inaccurately interpreted as part of the albedo, compromising the quality of relighting.

\begin{figure}[t!]
\centering
\includegraphics[width=0.9\linewidth]{./fig/application.png}
%\vspace{-0.5cm}
\caption{\textbf{Shadow removal can benefit indoor scene editing.}}
\vspace{-0.2cm}
\label{fig:application} 
\end{figure}

\subsection{Application 1: texture editing with shadow preservation.}

This application is grounded in the concept that while modifying the texture and keeping the geometry and light sources unchanged, preserving shadows is crucial for maintaining realism. The outcomes of this application, showcased in Fig.~\ref{fig:supp_app_1}, illustrate successive texture modifications while preserving the original shadows.

Specifically, given an input image, our process first perform shadow removal and detection using our method. Subsequently, we utilize the ControlNet conditioned on soft edges\cite{zhang2023adding} to generate an image with altered textures. The soft edges are extracted on the predicted shadow-free image, ensuring the preservation of geometry. Following this, we perform shadow removal once more using our proposed shadow removal network. Finally, by reintegrating the detected shadow probability map, we achieve texture editing while preserving original shadows (Fig.~\ref{fig:supp_app_1}).

\begin{figure}[t]
\centering
\includegraphics[width=\linewidth]{./fig/supp_app_1.jpg}
\caption{\textbf{Application 1: texture editing with shadow preservation.}}
\label{fig:supp_app_1} 
\end{figure}
\begin{figure}[t]
\centering
\includegraphics[width=\linewidth]{./fig/supp_app_2.jpg}
\caption{\textbf{Application 2: albedo estimation and relighting.} The shadow areas incorrectly estimated as part of the albedo are highlighted by the red arrows.}
\label{fig:supp_app_2} 
\end{figure}

\subsection{Application 2: albedo estimation and relighting.}

A crucial challenge in intrinsic image decomposition and material estimation~\cite{li2018learning,li2022physically,nestmeyer2020learning,ye2023intrinsicnerf} lies in classifying shadows and albedos. As shown in Fig.~\ref{fig:supp_app_2}, our shadow removal network can help resolve the ambiguities, thereby enhancing the quality of image editing applications.

Specifically, we leverage the approach in \cite{li2022physically} for single-image albedo estimation and relighting. This method predicts depth, normal, albedo, and roughness based on the RGB image. Subsequently, we manually position an area light and synthesize relit outputs using the neural renderer described in \cite{li2022physically}, comprising three modules: direct shading, direct shadow, and indirect shading. As depicted in Fig.~\ref{fig:supp_app_2}, without shadow removal, some shadows within the image might be misclassified as albedo. The presence of these shadows in the original image introduces artifacts in the relit results (Fig.\ref{fig:supp_app_2}).

It's important to note that the relighting quality in Fig.~\ref{fig:supp_app_2} may not be optimal due to the inaccuracies and low resolution of the predicted depth, normal, albedo, and roughness. However, despite these limitations, the outcomes obtained from albedo estimation and relighting serve to highlight the importance of our shadow removal technique in image editing.

% ###### SBUNewTest
% 阈值 0.1
% BER: 5.05, pErr: 7.63, nErr: 2.46, acc:0.9642
